# Supplementary material for: Quantifying the relationship between student enrollment patterns and student performance
Source: arXiv:2003.10874 source file (2020-11-08)
Supplement: Supplementary file 1 [file appendix_c.tex]

\section*{Appendix C}

As it is mentioned earlier, we applied the absorbing Markov model to compute the graduation rate. This approach is a special type of Markov chain in which the number of states is finite. Each absorbing Markov chain with t transient states and r absorbing states has a canonical form presented in matrix \ref{eq:Transition_Mat}. In the matrix, I is $r\times r$ identity matrix, O is $r\times t$ zero matrix, R is $t\times r$ matrix that represents a transition from the transient states to the absorbing states, and finally, Q is $t\times t$ matrix that expresses transitions between the transient states.

\begin{equation}P=\begin{bmatrix} \label{eq:Transition_Mat} 
Q~~ & R \\
O ~~& I \\
\end{bmatrix}\end{equation}

Each absorbing Markov Chain has two important characteristics: expected time until absorption (U) and probabilities of absorption (B) to the absorbing states. These characteristics are computed with Equations \ref{eq:U_Mat} and \ref{eq:B_Mat}. 
\begin{equation} \label{eq:U_Mat}
    U=N\times 1
\end{equation}
\begin{equation} \label{eq:B_Mat}
    B=N\times R
\end{equation}
where \begin{equation*} \label{eq:Fundemental_Mat}
    N=(I-Q)^{-1}
 \end{equation*}
In this problem, the transient states include one dummy state denoting \emph{new students} and four academic level states consisting \emph{Freshman}, \emph{Sophomore}, \emph{Junior}, and \emph{Senior}. The two absorbing states are whether or not students graduate. Each student first goes to the \emph{new student} state and then, based on his academic level, goes to the next corresponding state (For instance, a transferred student who starts his education at UCF with junior academic level has a transition from \emph{new student} state to \emph{junior} state). A transition will occur at the end of each semester based on the students' performance during the semester, which is the students' cumulative credits. Transition matrix alongside Markov diagram for FTIC student with full-time enrollment strategy are shown in Equation \ref{eq:Transition_Mat_FTIC} and \figref{fig:Transition_flow}. Using Equations \ref{eq:U_Mat} and \ref{eq:B_Mat}, the expected time until absorption (U) and the probabilities of absorption (B) for FTIC students with full-time enrollment strategy are shown in \tabref{tab:Time_to_G_H_FES_FTIC}. Since Equation \ref{eq:U_Mat} computes the expected time until absorption as the average time to graduate and time to halt, in order to obtain these times separately, we have computed U for students who graduate and halt separately.   

\begin{equation}P=\begin{bmatrix} \label{eq:Transition_Mat_FTIC} 
0 ~~& 0.85 ~~& 0.11 ~~& 0.04 ~~& 0    ~~& 0    ~~& 0 \\
0 ~~& 0.57 ~~& 0.35 ~~& 0    ~~& 0    ~~& 0.08 ~~& 0 \\
0 ~~& 0    ~~& 0.59 ~~& 0.35 ~~& 0    ~~& 0.06 ~~& 0 \\
0 ~~& 0    ~~& 0    ~~& 0.61 ~~& 0.36 ~~& 0.03 ~~& 0 \\
0 ~~& 0    ~~& 0    ~~& 0    ~~& 0.72 ~~& 0.01 ~~& 0.27 \\
0 ~~& 0    ~~& 0    ~~& 0    ~~& 0    ~~& 1    ~~& 0 \\
0 ~~& 0    ~~& 0    ~~& 0    ~~& 0    ~~& 0    ~~& 1 \\
\end{bmatrix}\end{equation}

\begin{figure}[!h]
\centering
  \includegraphics[width=0.75\textwidth]{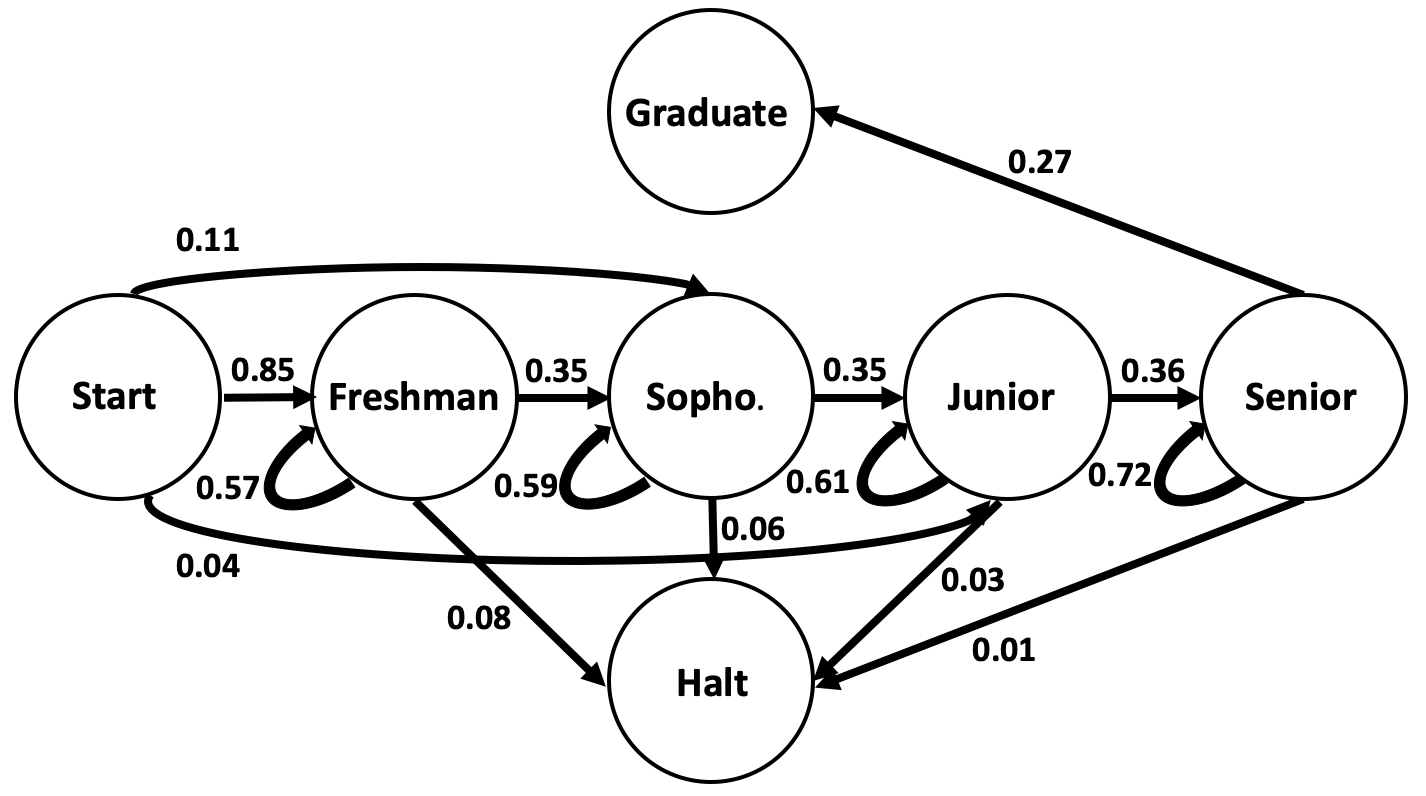}
\caption{Markov chain transitions probabilities for FES FTIC students}
\label{fig:Transition_flow}
\end{figure}

\begin{table}[!h]
\centering
% table caption is above the table
\caption{Graduation rate, time to graduate, and time to halt for FTIC students with full-time enrollment strategy }
\label{tab:Time_to_G_H_FES_FTIC}       % Give a unique label
% For LaTeX tables use
\begin{tabular}{llll}
\hline\noalign{\smallskip}
States&Graduation rate&Time to graduate&Time to halt\\
\noalign{\smallskip}\hline\noalign{\smallskip}
Start  & ~~~~~~~~74\%&~~~~~~~~~7.08&~~~~~~3.68 \\
Freshman  & ~~~~~~~~58\%&~~~~~~~~~8.28&~~~~~~3.01 \\
Sophomore & ~~~~~~~~62\%&~~~~~~~~~7.88&~~~~~~2.74 \\
Junior &~~~~~~~~73\%&~~~~~~~~~6.27&~~~~~~2.69 \\
Senior &~~~~~~~~89\%&~~~~~~~~~3.82&~~~~~~2.51 \\
\noalign{\smallskip}\hline
\end{tabular}
\end{table}
